# Supplementary material for: Generating Two-dimensional Ferromagnetic Charge Density Waves via External Fields
Source: arXiv:2204.11179 source file (2022-04-24)
Supplement: Supplementary file 1 [file SM-4.8.pdf]

# Supplemental Material for "Generating Two-dimensional Ferromagnetic Charge Density Waves via External Fields"

Heng Jin,[1] Jiabin Chen,[1] Yang Li,[1] Bin Shao,[2] and Bing Huang[1,3]

[1]*Beijing Computational Science Research Center, Beijing 100193, China*
[2]*College of Electronic Information and Optical Engineering, Nankai University, Tianjin 300350, China*
[3]*Department of Physics, Beijing Normal University, Beijing 100875, China*

## I. METHODS

**1. DFT Calculations.** Our first-principles calculations are performed using Vienna *ab initio* simulation package (VASP) [1] with projector augmented wave method (PAW) [2]. The exchange-correlation term is treated with the Perdew-Burke-Ernzerhof (PBE) form of the generalized gradient approximation [3]. The $3p^63d^44s^1$ and the $4s^24p^4$ electrons are treated as valence electrons for V and Se, respectively. A vacuum layer of 15 Å is introduced to avoid the interlayer interaction and simulate monolayer (ML) 1T-$VSe_2$. A Gaussian smearing of 0.05 eV has been adopted in our calculations. Energy cutoff of 500 eV and k mesh of $18 \times 18 \times 1$ over the Brillouin zone (BZ) have been chosen for geometry optimization of ML 1T-$VSe_2$. All structures are fully relaxed until force on each atom is less than 0.002 eV/Å. For static calculations, the energy cutoff of 600 eV, k mesh of $36\times36\times1$ over BZ and convergence criterion of total energy of $10^{-7}$ eV are used for the ML 1T-$VSe_2$, respectively. Our test calculations confirm that the spin orbital coupling (SOC) effect, which is not included in our study except for the calculation of magnetocrystalline anisotropic energy (MAE), will not influence our main conclusion. Similar k-spacing, energy cutoff and force convergence criterion have been adopted in the calculation of various CDW structures. We have fully tested the total energy convergence for all these 1T and CDW structures.

The simulation of in-plane biaxial strain is based on $\varepsilon = (a - a_0)/a_0$, where $a_0 = 3.34$ Å is the calculated lattice constant of unstrained ML 1T-$VSe_2$, in good agreement with experimentally reported value 3.35 Å [4]. Besides, our calculated band structure of 1T phase is also in accordance with APRES measurements [5, 6], indicating the accuracy and reliability of the computational method and our selected computational parameters. The Fermi surface is calculated with WANNIER90 software package [7]. Band unfolding is performed with BANDUP code [8, 9]. The phonon spectra of ML 1T-$VSe_2$, $\sqrt{3}\times\sqrt{3}$ and $2\times2\sqrt{3}$ ferromagnetic CDWs are calculated based on $8\times8\times1$, $2\times2\times1$ and $2\times2\times1$ supercells respectively with finite displacement method [10], as implemented in PHONOPY software [11] with precision consistent with geometry relaxation. For a detailed discussion about the origins of half-metallic CDWs, the Quantum Espresso (QE) software package [12] is used to calculate phonon linewidth. We use ultrasoft pseudopotentials in the QE calculations. The k mesh of $32\times32\times1$ and q mesh of $8\times8\times1$ are adopted and the energy cutoff of wave function (charge density) is set to 70 (700) Ry., which is sufficiently high to obtain the converged results.

**2. Electron Susceptibility Calculations.** The nesting function as the low-frequency limit of the imaginary part of electron susceptibility is calculated based on the following expression:

$$\mathrm{Im}\chi_{\boldsymbol{q}} = \sum_{\boldsymbol{k}} \delta\left(\varepsilon_{\boldsymbol{k}} - \varepsilon_F\right)\delta\left(\varepsilon_{\boldsymbol{k}+\boldsymbol{q}} - \varepsilon_F\right) \tag{1}$$

in which $\delta(x)$ is numerically approximated by

$$\delta(x) \approx \frac{1}{\pi}\frac{\epsilon}{\epsilon^2 + x^2} \tag{2}$$

with $\epsilon = 0.02$. The real part of electron susceptibility is calculated by

$$\mathrm{Re}\chi_{\boldsymbol{q}} = \sum_{\boldsymbol{k}} \frac{f\left(\varepsilon_{\boldsymbol{k}}\right) - f\left(\varepsilon_{\boldsymbol{k}+\boldsymbol{q}}\right)}{\varepsilon_{\boldsymbol{k}} - \varepsilon_{\boldsymbol{k}+\boldsymbol{q}}} \tag{3}$$

reflecting the stability of the electronic system[13, 14]. The $\varepsilon_{\boldsymbol{k}}$ is the eigenvalue of Kohn-Sham equation, $\varepsilon_F$ the Fermi level, and $f$ the Fermi-Dirac distribution function.

**3. Phonon linewidth calculations.** We calculate phonon linewidth $\gamma$ as

$$\gamma_{\boldsymbol{q}} = 2\pi\omega(\boldsymbol{q}) \int \frac{d\boldsymbol{k}}{\Omega_{BZ}} |g(\boldsymbol{k},\boldsymbol{q})|^2 \delta\left(\varepsilon_{\boldsymbol{k}} - \varepsilon_F\right)\delta\left(\varepsilon_{\boldsymbol{k}+\boldsymbol{q}} - \varepsilon_F\right) \tag{4}$$

where the integration is over BZ. The $\Omega_{BZ}$ is the area of BZ and $g(\boldsymbol{k}, \boldsymbol{q})$ is the electron-phonon coupling matrix. Since different pseudopotentials are adopted for the calculations of phonon spectra (in VASP) and phonon linewidths (in QE), we have tested the phonon spectra using both methods (e.g., see Fig. S8), which shows a good agreement with each other.

## II. SUPPLEMENTAL TABLES AND FIGURES

**1. Relations between CDWs and dynamical instability in phonon spectrum of monolayer (ML) 1T-$VSe_2$.** The relationships between primitive cell and supercells are summarized in Tab. S1. In our calculations, we choose primitive cell of 1T-$VSe_2$ with angle between two lattice vectors being 120°. The lattice vectors of reciprocal lattice of supercells are marked as $\boldsymbol{q_1}$ and $\boldsymbol{q_2}$. The instabilities in phonon spectrum of 1T-$VSe_2$ would fold to Γ as softened optical modes if corresponding supercell is adopted. Therefore, the instabilities in phonon spectrum of 1T-$VSe_2$ indicate CDWs where structure reconstructions take place in their corresponding supercells.

| | $2\times2$ | $4\times4$ | $2\times2\sqrt{3}$ | $\sqrt{3}\times\sqrt{3}$ | $\sqrt{7}\times\sqrt{3}$ |
|---|---|---|---|---|---|
| $\boldsymbol{a}'$ | $2\boldsymbol{a}$ | $4\boldsymbol{a}$ | $2\boldsymbol{a}$ | $2\boldsymbol{a}+\boldsymbol{b}$ | $3\boldsymbol{a}+2\boldsymbol{b}$ |
| $\boldsymbol{b}'$ | $2\boldsymbol{b}$ | $4\boldsymbol{b}$ | $\boldsymbol{2a+4b}$ | $\boldsymbol{a}+2\boldsymbol{b}$ | $-\boldsymbol{a}+\boldsymbol{b}$ |
| $\boldsymbol{q_1}$ | $\frac{1}{2}\boldsymbol{a}^*\,(M)$ | $\frac{1}{4}\boldsymbol{a}^*\,\left(\frac{1}{2}\Gamma-M\right)$ | $\frac{1}{2}\boldsymbol{a}^*-\frac{1}{4}\boldsymbol{b}^*\,\left(\frac{3}{4}\Gamma-K\right)$ | $\frac{2}{3}\boldsymbol{a}^*-\frac{1}{3}\boldsymbol{b}^*\,(K)$ | $\frac{1}{5}\boldsymbol{a}^*+\frac{1}{5}\boldsymbol{b}^*\,\left(\frac{3}{5}\Gamma-K\right)$ |
| $\boldsymbol{q_2}$ | $\frac{1}{2}\boldsymbol{b}^*\,(M)$ | $\frac{1}{4}\boldsymbol{b}^*\,\left(\frac{1}{2}\Gamma-M\right)$ | $\frac{1}{4}\boldsymbol{b}^*\,\left(\frac{1}{2}\Gamma-M\right)$ | $-\frac{1}{3}\boldsymbol{a}^*+\frac{2}{3}\boldsymbol{b}^*\,(K)$ | $-\frac{2}{5}\boldsymbol{a}^*+\frac{3}{5}\boldsymbol{b}^*\,\left(\frac{9}{5}\Gamma-K\right)$ |

Table S1. Lattice vectors of CDWs and ML 1T-$VSe_2$ in real space and reciprocal space. $\boldsymbol{a}$ and $\boldsymbol{b}$ are lattice vectors of primitive cell of 1T-$VSe_2$ with an angle 120Å. $\boldsymbol{a}'$ and $\boldsymbol{b}'$ are lattice vectors of CDWs. $\boldsymbol{q_1}(\boldsymbol{a}^*)$ and $\boldsymbol{q_2}(\boldsymbol{b}^*)$ are lattice vectors of CDWs (ML 1T-$VSe_2$) in reciprocal space. Symbols in brackets indicate the location of dynamic instabilities corresponding to CDW formations in phonon spectrum of 1T-$VSe_2$.

**2. Dynamical instabilities of nonmagnetic ML 1T-$VSe_2$ under different strain.** As is shown in Fig. S1, under $\varepsilon = 0\%$ two distinct instabilities locate near $1/2\ \Gamma{-}M$ and $3/5\ \Gamma-K$. Interestingly, the enhanced instabilities in phonon spectra are observed with increasing tensile strain.

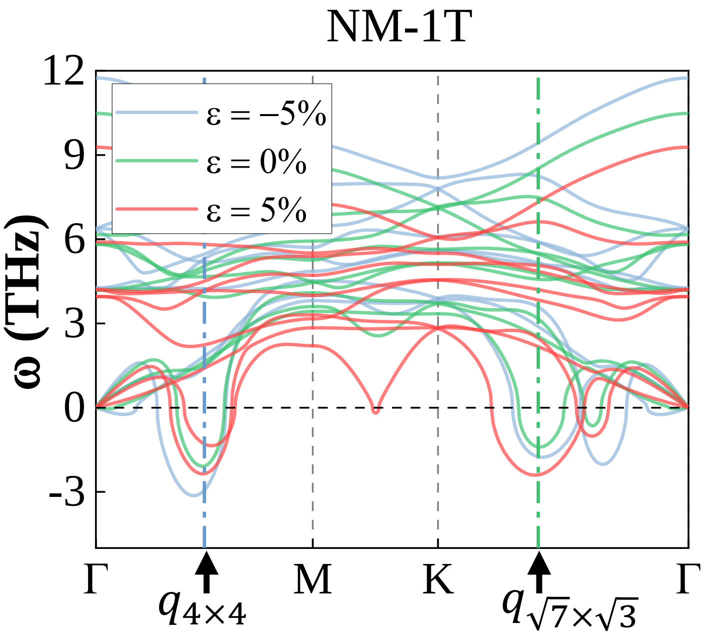


Figure S1. Phonon spectra of nonmagnetic (NM) ML 1T-$VSe_2$ under three different strains. These instabilities corresponding to $4 \times 4$ and $\sqrt{7} \times \sqrt{3}$ CDWs are marked with arrows.

**3. Dynamical stability of $2 \times 2\sqrt{3}$ and $\sqrt{3} \times \sqrt{3}$ ferromagnetic CDWs.** As shown in Fig. S2, the phonon spectra of $2 \times 2\sqrt{3}$ and $\sqrt{3} \times \sqrt{3}$ ferromagnetic (FM) CDWs are calculated under $\varepsilon = 5\%$ within $2 \times 2$ supercells. In addition, the phonon spectrum of $\sqrt{3} \times \sqrt{3}$ FM CDW under $\varepsilon = 3\%$ is also checked to be dynamically stable (not show here).

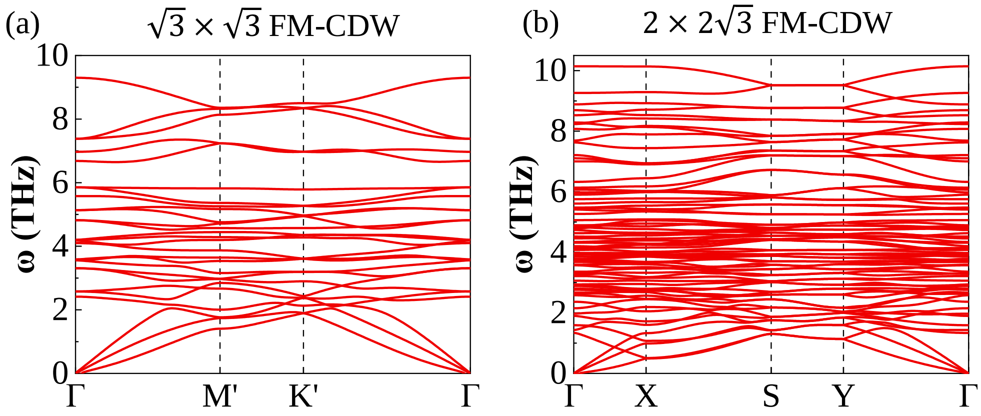


Figure S2. (a) and (b) Phonon spectra of $\sqrt{3} \times \sqrt{3}$ and $2 \times 2\sqrt{3}$ FM CDWs calculated within a $2 \times 2$ supercell under $\varepsilon = 5\%$, respectively.

**4. Antiferromagnetic configurations of CDWs.** To investigate the stability of long-range FM order of the CDWs, two typical antiferromagnetic (AFM) configurations are set as initial magnetic configurations (see Fig. S3) and atoms are fully relaxed before the calculation of their total energies. The MAE is also calculated with consideration of SOC effect. Here, MAE is evaluated by the energy difference between in-plane and out-of-plane spin configurations, and the positive values in Table S2 mean the easy axis of both CDWs is along the in-plane direction. We emphasize that our calculations indicate that the MAE along in-plane $x$-axis and $y$-axis are very close to each other. Our results

suggest the existence of long-range FM order.

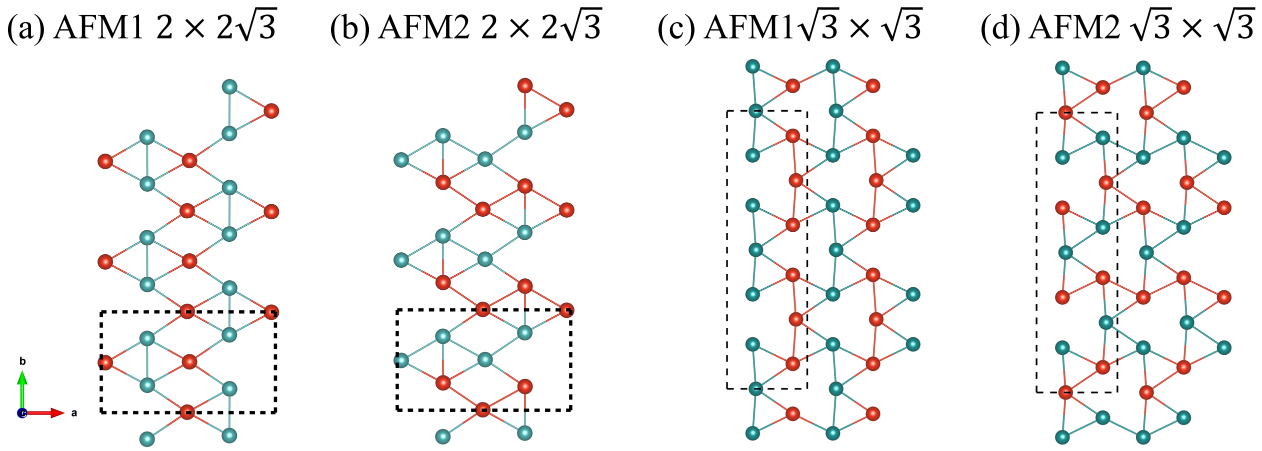


Figure S3. (a) and (b) Two AFM configurations of $2 \times 2\sqrt{3}$ CDW. (c) and (d) Two AFM configurations of $\sqrt{3} \times \sqrt{3}$ CDW. Only V atoms are plotted for simplicity and spins of opposite orientations are marked by two different colors. Supercells to accommodate AFM configurations are illustrated with dashed lines.

| | strain | $E_{AFM1}$-$E_{FM}$(meV/f.u.) | $E_{AFM2}$-$E_{FM}$(meV/f.u.) | MAE (meV/f.u.) |
|---|---|---|---|---|
| $\sqrt{3} \times \sqrt{3}$ | 3% | 43.6 | 19.7 | 0.18 |
| | 5% | 64.5 | 30.4 | 0.21 |
| $2 \times 2\sqrt{3}$ | 3% | 26.3 | 10.7 | 0.36 |
| | 5% | 48.8 | 22.7 | 0.51 |

Table S2. Energy difference between FM and AFM states and magnetocrystalline anisotropy energy (MAE) of CDWs under different strain.

**5. Electronic structures of $2 \times 2\sqrt{3}$ FM CDW under different tensile strain.** The spin-resolved density of states (DOS) of $2 \times 2\sqrt{3}$ FM CDW under different tensile strain is shown in Fig. S4, as a detailed illustration for the evolution of spin polarization ratio $P$ in Fig. 2(e) in the main text. When the tensile strain increases, the bandgap in spin $\uparrow$ channel gradually decreases and eventually closes, while the bandgap in spin $\downarrow$ channel gradually increases. The dramatically different evolutions in different spin channels result in $P$ gradually changing from negative ($\sim -90\%$ ) to positive ($\sim +100\%$). Again, we emphasize here that the different spin channels are distinguishable using the spin-polarized STM measurements, as shown in Fig. S5.

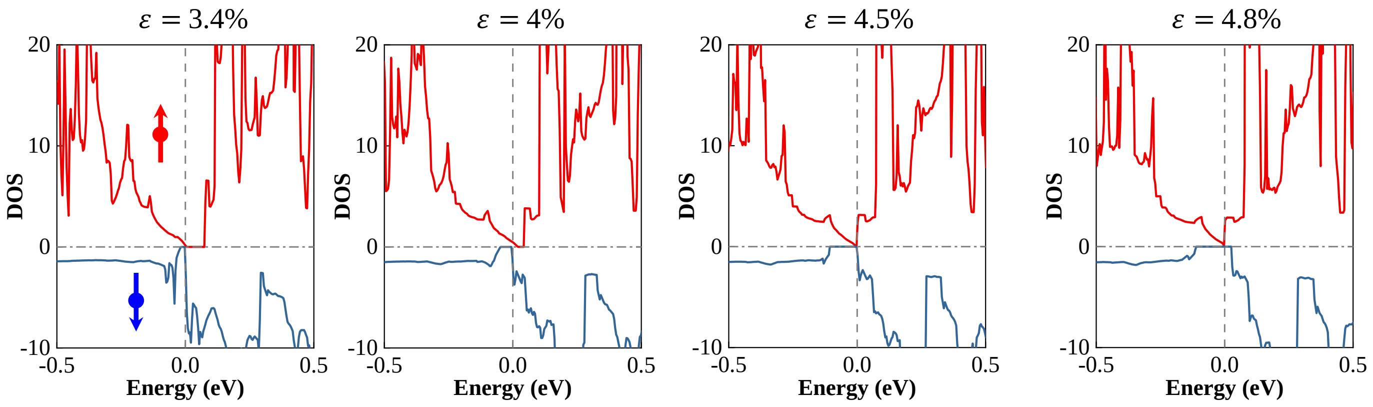


Figure S4. Spin-resolved DOS of the $2 \times 2\sqrt{3}$ FM CDW phase under different strain.

**6. Spin-polarized STM simulations.** In experiments, spin-resolved STM [15] is available to identify these two dramatically different half-metallic CDWs. To simulate the STM dI/dV mapping, local DOS (LDOS) in the plane of $\sim 3$ Å above the outmost Se-terminated surface has been calculated; for each bias voltage $V_b$, LDOS is integrated in energy range of $V_b \pm 25$ meV. Fig. S5(a) shows the simulated STM images of $\sqrt{3} \times \sqrt{3}$ half-metallic CDW ($\varepsilon = 3\%$). When $V_b = 0$ meV, the spin $\downarrow$ channel exhibits $Se_1$-formed bright hexagon spots, but nothing can be resolved in spin $\uparrow$ channel, reflecting an A-type half-metallic feature. The case is opposite for $2 \times 2\sqrt{3}$ half-metallic CDW ($\varepsilon = 5\%$). Under $V_b = 0$ meV, nothing can be resolved in spin $\downarrow$ channel, but the $Se_6$-formed bright rectangle spots are observable in spin $\uparrow$ channel [Fig. S5(b)], reflecting a B-type half-metallic feature.

Interestingly, the bright spots could dramatically shift to a different spin channel under $V_b$. For example, as shown in Fig. S5(a), when $V_b = -200$ (or $+200$) meV, the $Se_1$-formed bright hexagon spots are no longer visible in spin $\downarrow$ channel but visible in spin $\uparrow$ channel of $\sqrt{3} \times \sqrt{3}$ half-metallic CDW, due to much higher LDOS of $Se_1$ emerging in spin $\uparrow$ than in spin $\downarrow$ channel in this energy region. For $2 \times 2\sqrt{3}$ half-metallic CDW, as shown in Fig. S5(b), when $V_b = 200$ meV, the bright spots are no longer visible in spin $\uparrow$ channel, but the $Se_4$-formed rectangle spots appear in spin $\downarrow$ channel; when $V_b = -200$ meV, the bright spots in spin $\uparrow$ channel are still visible but formed by $Se_7$ and $Se_8$ atoms instead of $Se_4$ atoms. The simulated STM images along with the $V_b$-tunable bright-spot transitions in different spin channels can provide a clue to identify these half-metallic CDWs in the future experiments.

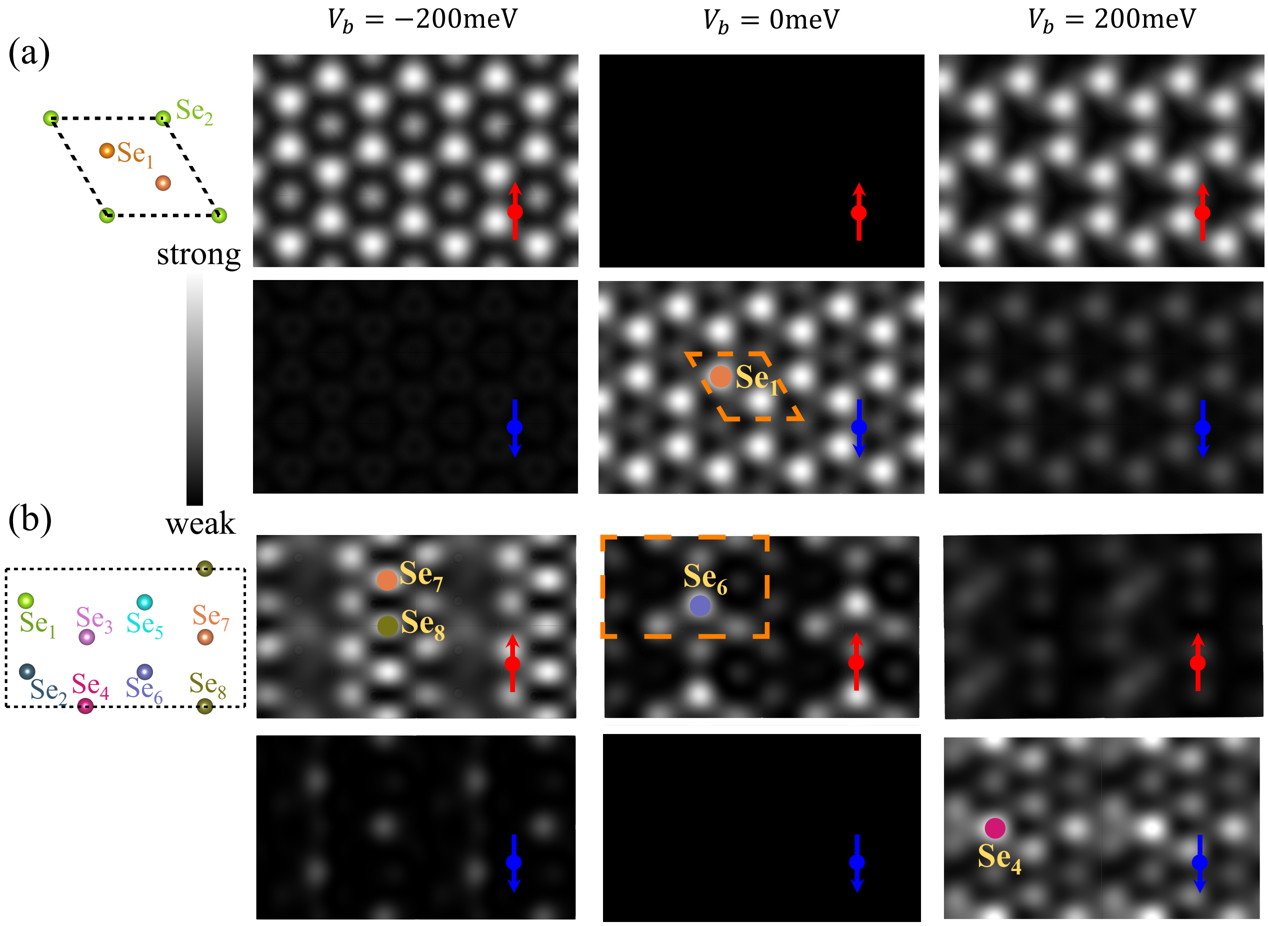


Figure S5. Spin-polarized STM simulations of (a) $\sqrt{3}\times\sqrt{3}$ CDW under $\varepsilon = 3\%$ and (b) $2\times 2\sqrt{3}$ CDW under $\varepsilon = 5\%$. The primitive cell is illustrated with dashed-lines. Left panels label all inequivalent Se atoms. For simplicity only Se atoms of top layer are shown.

**7. Tunable flat-band positions in $\sqrt{3}\times\sqrt{3}$ FM CDW by strain and electron doping.** As shown in Fig. S6, the Fermi level of $\sqrt{3}\times\sqrt{3}$ CDW can be tuned to close the flat band with 5% tensile strain (Fig. S6(a)), and cross the flat-band with the additional moderate electron doping (Fig. S6(b)), providing $\sqrt{3}\times\sqrt{3}$ FM CDW as promising candidate for studying flat-band-related strongly correlated physics.

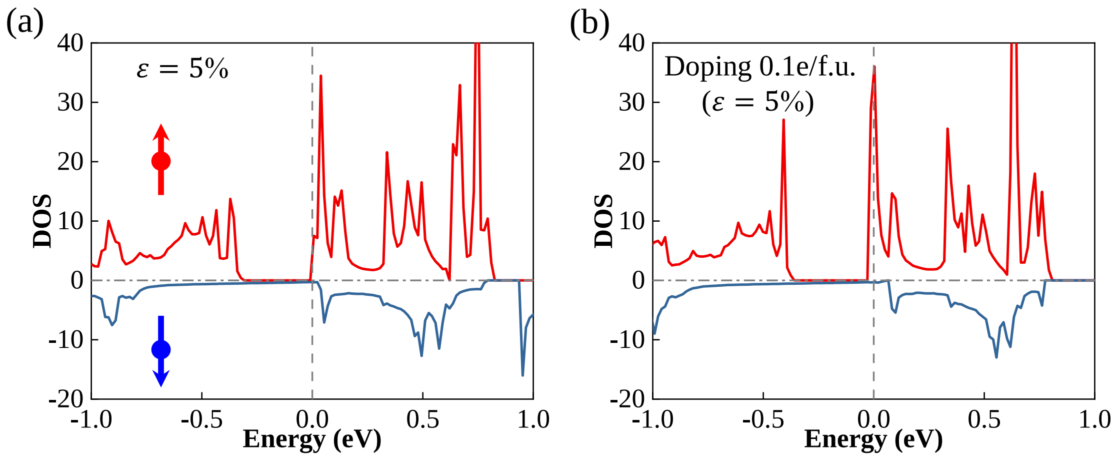


Figure S6. (a) DOS of $\sqrt{3}\times\sqrt{3}$ FM CDW under $\varepsilon = 5\%$. (b) DOS of $\sqrt{3}\times\sqrt{3}$ FM CDW under $\varepsilon = 5\%$ and additional electron doping 0.1 e/f.u..

**8. Real part of electron susceptibility under different strain.** As shown in Fig. S7(a), the real part of electron susceptibility Re$\chi$ shows intensive peaks at $K$ point, in agreement with the peaks of Im$\chi$ [see Fig. 4(a)]. This suggests the strong Fermi surface nesting of the spin $\uparrow$ channel at $K$ under $\varepsilon = 3\%$. Hence, the origin of $\sqrt{3}\times\sqrt{3}$ FM CDW involves the Fermi surface nesting of spin $\uparrow$ channel.

On the contrary, under $\varepsilon = 5\%$, Re$\chi$ of both spin channels (see Fig. S7(c) and Fig. S7(d)) show major peaks around $M$, suggesting strong instability of electronic systems which indicates a $2\times 2$ CDW rather than a $2\times 2\sqrt{3}$ CDW. Therefore, the Fermi surface nesting of both spin channels does not contribute the formation of $2\times 2\sqrt{3}$ FM CDW under $\varepsilon = 5\%$.

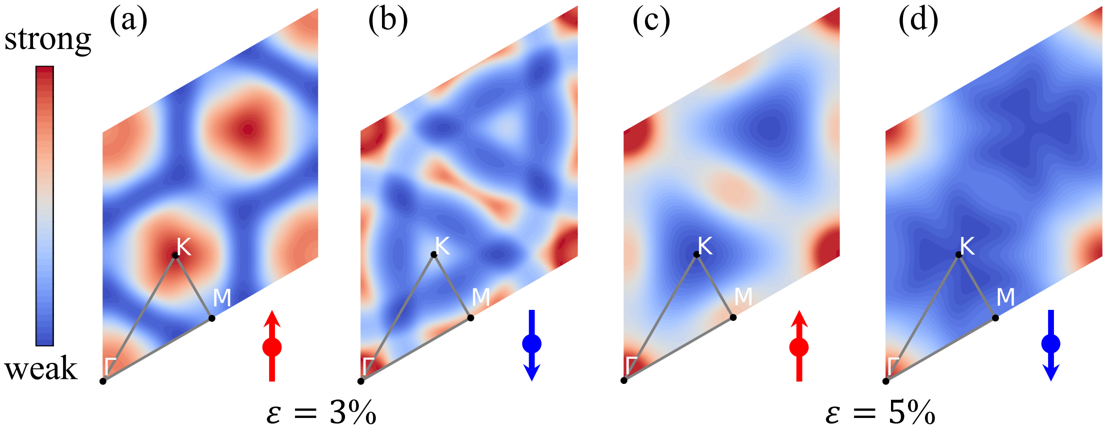


Figure S7. Real part of electron susceptibility (Re$\chi$) under different strain. (a) spin $\uparrow$ channel and (b) spin $\downarrow$ channel under $\varepsilon = 3\%$. (c) spin $\uparrow$ channel and (d) spin $\downarrow$ channel under $\varepsilon = 5\%$. The color bar is different for each picture.

**9. Phonon spectra calculated using ultrasoft pseudopotential (US) and PAW methods.** As is shown in Fig. S8, the phonon spectra of FM ML 1T-$VSe_2$ are calculated with both ultrasoft pseudopotential and PAW method. In general PAW method and ultrasoft pseudopotential are in good agreement with each other describing the properties of phonons. Since the properties of phonon can be also well described by ultrasoft pseudopotential, the phonon linewidths calculated with ultrasoft pseudopotential should be valid consistently.

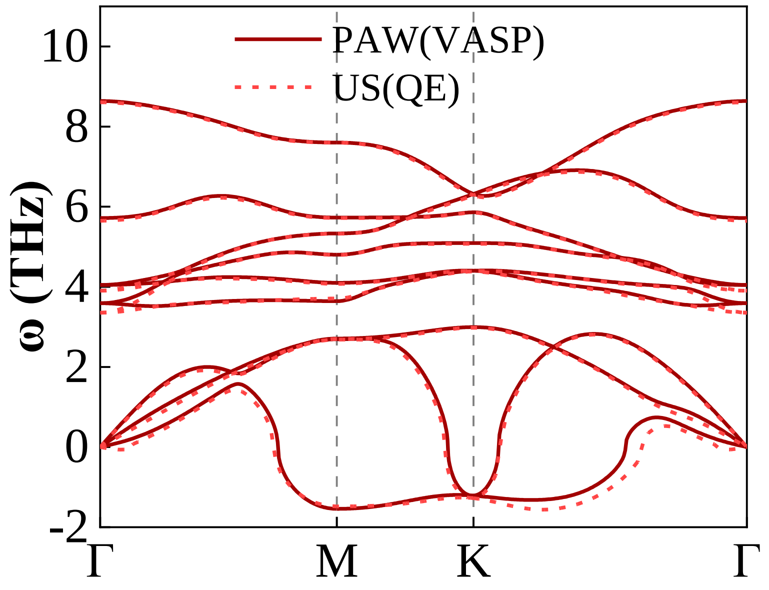


Figure S8. Phonon spectra of ferromagnetic 1T-VSe$_2$ using ultrasoft pseudopotential (US) and PAW methods under $\varepsilon = 5\%$.

[1] G. Kresse and J. Furthmüller, Phys. Rev. B **54**, 11169 (1996).

[2] P. E. Blöchl, Phys. Rev. B **50**, 17953 (1994).

[3] J. P. Perdew, K. Burke, and M. Ernzerhof, Phys. Rev. Lett. **77**, 3865 (1996).

[4] W. Yu, J. Li, T. S. Herng, Z. Wang, X. Zhao, X. Chi, W. Fu, I. Abdelwahab, J. Zhou, J. Dan, Z. Chen, Z. Chen, Z. Li, J. Lu, S. J. Pennycook, Y. P. Feng, J. Ding, and K. P. Loh, Adv. Mater. **31**, 1903779 (2019).

[5] P. Chen, W. W. Pai, Y.-H. Chan, V. Madhavan, M. Chou, S.-K. Mo, A.-V. Fedorov, and T.-C. Chiang, Phys. Rev. Lett. **121**, 196402 (2018).

[6] P. M. Coelho, K. N. Cong, M. Bonilla, S. Kolekar, M.-H. Phan, J. Avila, M. C. Asensio, I. I. Oleynik, and M. Batzill, J. Phys. Chem. C **123**, 14089 (2019).

[7] A. A. Mostofi, J. R. Yates, G. Pizzi, Y.-S. Lee, I. Souza, D. Vanderbilt, and N. Marzari, Comput. Phys. Commun. **185**, 2309 (2014).

[8] P. V. C. Medeiros, S. Stafström, and J. Björk, Phys. Rev. B **89**, 041407 (2014).

[9] P. V. C. Medeiros, S. S. Tsirkin, S. Stafström, and J. Björk, Phys. Rev. B **91**, 041116 (2015).

[10] K. Kunc and R. M. Martin, Phys. Rev. Lett **48**, 406 (1982).

[11] A. Togo and I. Tanaka, Scr. Mater. **108**, 1 (2015).

[12] P. Giannozzi, S. Baroni, N. Bonini, M. Calandra, R. Car, C. Cavazzoni, D. Ceresoli, G. L. Chiarotti, M. Cococcioni, I. Dabo, A. D. Corso, S. de Gironcoli, S. Fabris, G. Fratesi, R. Gebauer, U. Gerstmann, C. Gougoussis, A. Kokalj, M. Lazzeri, L. Martin-Samos, N. Marzari, F. Mauri, R. Mazzarello, S. Paolini, A. Pasquarello, L. Paulatto, C. Sbraccia, S. Scandolo, G. Sclauzero, A. P. Seitsonen, A. Smogunov, P. Umari, and R. M. Wentzcovitch, J. Phys.: Condens. Matter **21**, 395502 (2009).

[13] M. D. Johannes and I. I. Mazin, Phys. Rev. B **77**, 165135 (2008).

[14] J. G. Si, W. J. Lu, H. Y. Wu, H. Y. Lv, X. Liang, Q. J. Li, and Y. P. Sun, Phys. Rev. B **101**, 235405 (2020).

[15] R. Wiesendanger, Rev. Mod. Phys. **81**, 1495 (2009).
